# Supplementary material for: Heterogeneous cavitation from atomically smooth liquid-liquid interfaces
Source: arXiv:2306.01571 source file (2023-06-02)
Supplement: Supplementary file 1 [file Suppl.pdf]

# Supplementary Material for Heterogeneous cavitation from atomically smooth liquid-liquid interfaces

Patricia Pfeiffer,[1,*] Meysam Shahrooz,[2] Marco Tortora,[2] Carlo Massimo Casciola,[2]
Ryan Holman,[3] Rares Salomir,[3,4] Simone Meloni,[5,†] and Claus-Dieter Ohl[1]

[1]*Institute of Physics, Otto-von-Guericke University Magdeburg, Universitätsplatz 2, 39106 Magdeburg, Germany*

[2]*Dipartimento di Ingegneria Meccanica e Aerospaziale - DIMA, University of Rome "Sapienza", via Eudossiana 18, 00158 Roma, Italy*

[3]*Image Guided Interventions Laboratory (GR-949), Faculty of Medicine, University of Geneva, Geneva, Switzerland*

[4]*Radiology Department, University Hospitals of Geneva, Geneva, Switzerland*

[5]*Dipartimento di Scienze Chimiche, Farmaceutiche e Agrarie - DOCPAS, University of Ferrara, via Luigi Borsari 46, 44121 Ferrara, Italy*

[*] patricia.pfeiffer@ovgu.de

[†] mlnsmn@unife.it

## I. MULTIPLE DROPLET CAVITATION

A droplet may nucleate multiple times. This is demonstrated in Fig. S1. Here, the PFC droplets marked in the upper row with a red circle at $t = 0$ are followed for a longer time until $t = 10.2\,\mu s$. Initially, we see that these two droplets nucleate a bubble at $t = 0.2\,\mu s$ that collapses and is not detected anymore after $t = 1.2\,\mu s$. At $t = 7.6\,\mu s$ the droplets have been displaced slightly to the right and at $t = 8.8\,\mu s$ they again nucleate a bubble. We speculate that reflections of waves within the glass result in this late rarefaction wave. This demonstrates that a droplet is not used up by one cavitation event but can serve multiple times as a cavitation nucleus. A word of caution, some unresolved gas bubbles may remain as a result of the first cavitation event, and this may nucleate the second cavitation event, too.

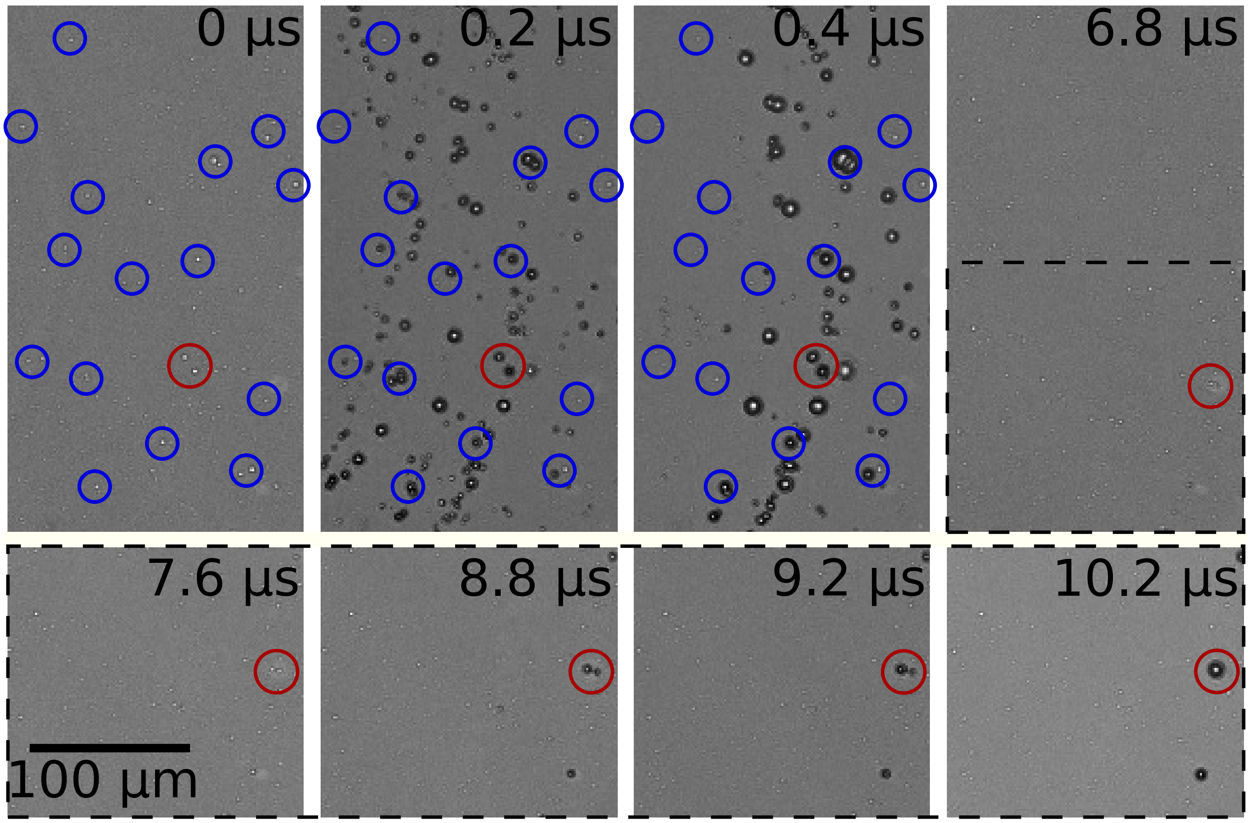


FIG. S 1. Multiple droplet cavitation. Experimental snapshots of cavitation nucleation in a PFOB emulsion. Some PFOB droplets are marked with a blue circle. At $t = 0.2 - 0.4\,\mu s$, i.e. when the Lamb wave passes, on most of these droplets a bubble is formed. The red circle marks two droplets, which show cavitation at $t = 0.2 - 0.4\,\mu s$. With time they are transported by the flow, created by the main bubble expansion towards the right ($t = 6.8 - 7.6\,\mu s$). At $t = 8.8\,\mu s$, on the very same droplets bubbles are formed again by a tension wave.

## II. SINGLE INTERFACE BUBBLE NUCLEATION

During preparation of the droplets through sonication particulate contamination may be generated, e.g. through sub-micrometer sized metal particles eroded from the ultrasonic horn. Those particles may remain in suspension and accumulate at the liquid-liquid interface.

To rule out that the cavitation is due to nanoparticles trapped at the liquid-liquid interface the sonication step was omitted. A clean liquid-liquid interface was created by depositing a macroscopic droplet of water and a droplet of PFOB side-by-side onto a microscope slide and covering them with a cover slip resulting in an interface without the possibility to entrap particles. The Lamb wave was generated then in a rather thick gap where the height was adjusted to 10 μm with suitable spacers. For this thickness the rarefaction wave does *not* nucleate cavitation in either of the two liquids.

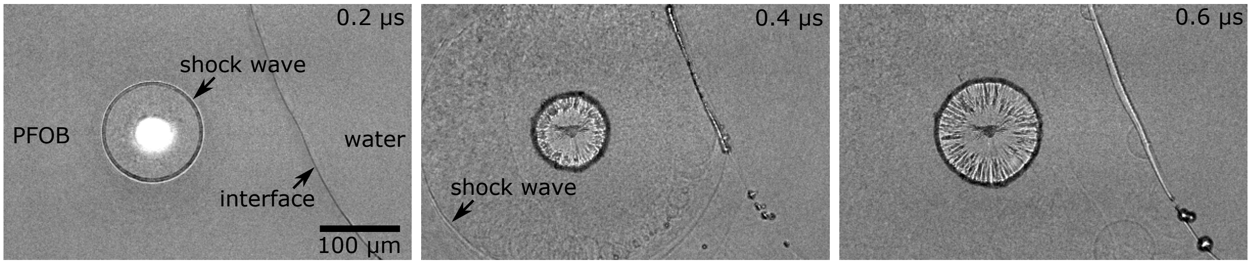


FIG. S 2. Cavitation activity near a PFOB-water interface in a liquid gap. Secondary cavitation bubbles are mainly formed at the interface.

Figure S2 depicts the course of events. At time $t = 0.2\,\mu s$ the plasma from the pulsed laser and the emitted shock wave are visible. Once the shock wave reaches the PFOB-water interface, $t = 0.4\,\mu s$, a line of cavitation bubbles nucleate at this interface and coalesce into a long thin strip of vapor. At $t = 0.6\,\mu s$ most bubbles have collapsed and due to the flow induced by the central bubble the liquid-liquid interface is displaced to the right.

The shape of the cavitation pattern supports the experimental interpretation and molecular dynamics simulation of having as supersaturated region between the liquids.

## III. GAS LAYER FORMATION AT THE WATER/PFC INTERFACE

The accumulation of $N_2$ molecules in the MD simulations are presented in Fig. S3. Here, the arrows marks the regions, where cavities in the water phase at the liquid-liquid interface occur due to the accumulation of gas molecules in this area.

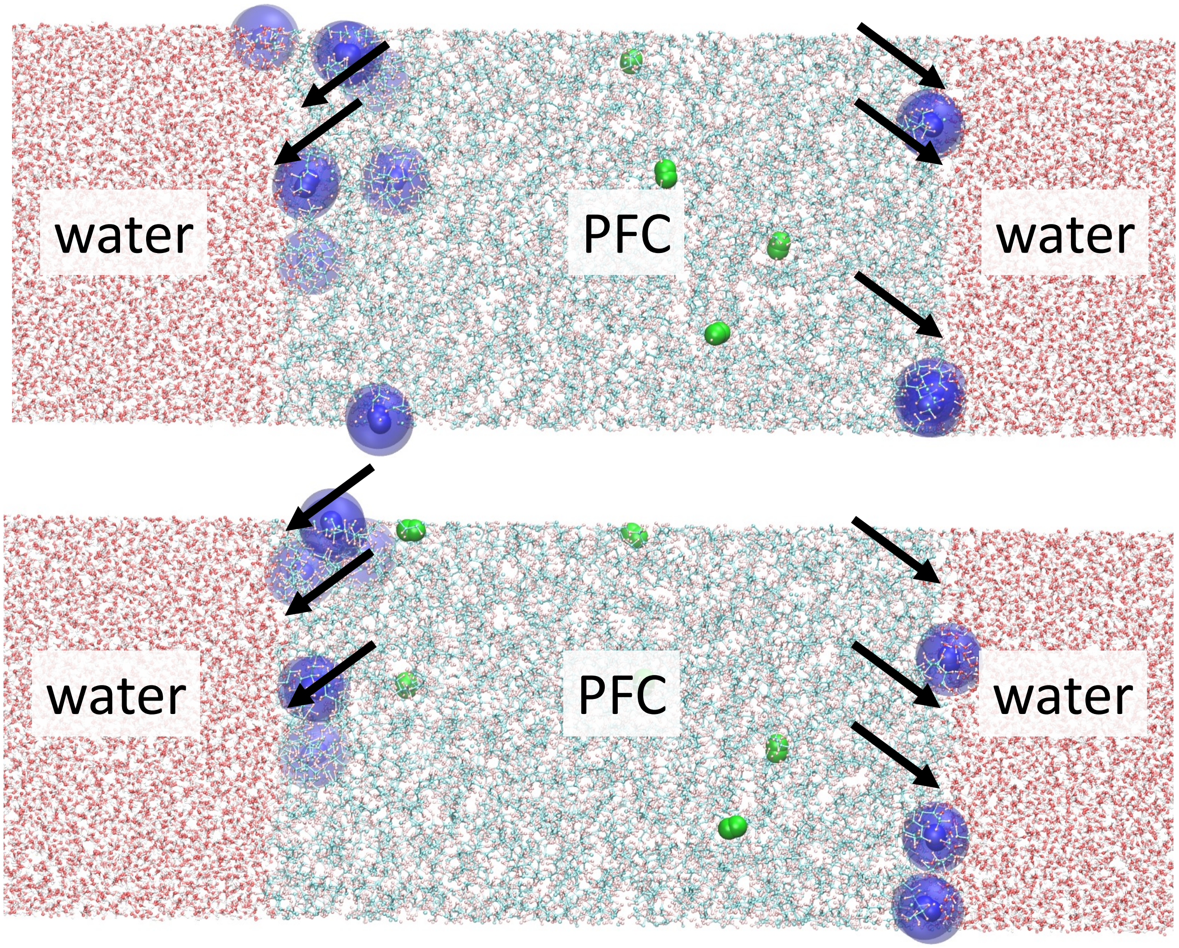


FIG. S 3. Two more snapshots of the atomistic sample illustrating the formation of a gas layer at the water/PFC interface. Blue spheres highlighted by a spherical shadow of the same color are *interface* nitrogen molecules, arbitrarily defined as those molecules within 2 nm of both water and PFC molecules, i. e., within 2 nm from the interface. The complementary bulk nitrogen molecules are represented as green spheres. The arrows show the opening of cavities in the water domain of the interface due to the presence of gas molecules. This is more visible in some cases as there are several molecules at a short distance from each other. In other cases, this is harder to appreciate as the gas molecules are deeper in the sample. A movie of a 1 ns branch of the MD trajectory at −20 MPa is provided in the Supplementary Materials.

## IV. EFFECT OF $N_2$ SUPERSATURATION ON THE PROPERTIES OF THE COMPUTATIONAL SAMPLE

In the main text we mentioned that in our simulations we used an $N_2$ gas concentration ∼5 times higher than the experimental saturation value, which helps obtaining reliable computational results within the timescale accessible to molecular dynamics. Here we support the reliability of this approach showing that on the timescale of simulations this oversaturation produces no artefacts in the computational sample.

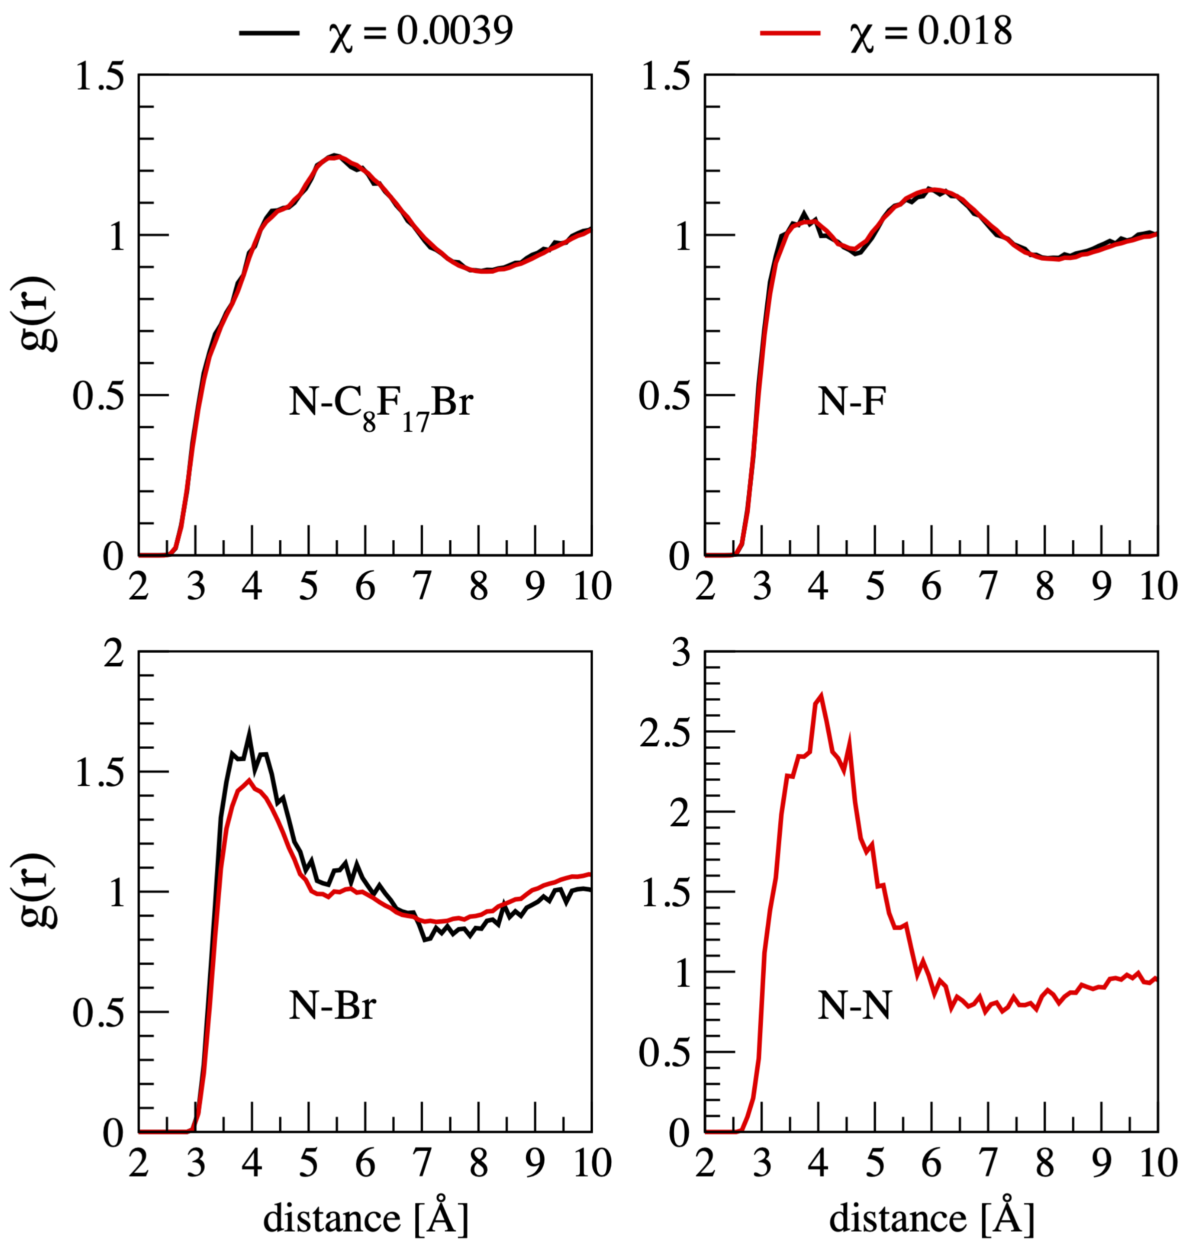


FIG. S 4. Comparison between (partial) pair correlation functions of two PFC/$N_2$ bulk samples at molar fraction $\chi = 0.0039$ (black), close to the experimental saturation concentration, and $\chi = 0.018$ (red), the concentration used in the water/PFC interface simulations. Top-left panel shows pair correlation function between atoms of the gas and atoms of PFC; top-right and bottom-left focus on N-F and N-Br pairs. Bottom-right panel shows the pair correlation function between nitrogen atoms belonging to different molecules.

Fig. S4 shows several partial pair correlation functions, $g(r)$, between $N_2$ and PFC - including the specific case of N-F and N-Br - and between $N_2$ molecules for two PFC/$N_2$ bulk samples at gas molar fraction $\chi = 0.0039$, close to the experimental saturation concentration [1], and $\chi = 0.018$, the concentration used in the water/PFC interface simulations. The pair correlation function represents the

probability (density) to find two atoms at distance $r$ in the system at hand with respect to the case of an uncorrelated system (ideal gas).

Concerning the partial $N_2$-PFC correlation functions (top row and bottom-left panels of Fig. S4), no significant differences between the two samples at different concentrations are observed, apart, as expected, a better statistic in the $\chi = 0.018$ case. Concerning the N-N pair correlation function (bottom-right panel of Fig. S4), for the low concentration solution $g(r) = 0$ in the range of intermolecular distances, i. e., beyond twice the N van der Waals radius. This is apparently surprising because even if there were no interaction between $N_2$ molecules the pair correlation function should be equal to 1 in this region. This, indeed, is an artefact of the insufficient simulation time to reproduce the fundamental structural properties of a highly diluted (gas) solute on the timescale of simulations, here 5 ns. On the contrary, the N-N pair correlation function of the $\chi = 0.018$ sample obtained by a simulation of the same duration shows the expected profile of a (concentrated) gas, with a peak corresponding to the first coordination shell quickly degrading to 1. Present results confirm the suitability of the "oversaturation" approach: the level of oversaturation considered in this work i) introduces no significant structural changes in the system while ii) allows to achieve well converged properties in short times, compatible with the timescale accessible to molecular dynamics.

## V. EFFECT OF $N_2$ SUPERSATURATION ON THE BUBBLE NUCLEATION BARRIER

To estimate the effect of local supersaturation on the bubble nucleation barrier, one can resort to the classical nucleation theory, as adapted by Lubetkin to the case of a supersaturated liquid [2]. Here, the nucleation rate $j$ depends exponentially on the barrier $\Delta G^\dagger$: $j = C \exp[-\Delta G^\dagger / k_B T]$, with $k_B$ the Boltzmann constant and $T$ the temperature of the system. For the pre-exponential factor $C$ several forms have been developed [3–5], which have been recently tested to be quantitatively accurate when tested against controlled *in silico* experiments [6]. The key conclusion to bear in mind is that with $\Delta G^\dagger \sim 5$ k$_B$T, i. e., 5 times the thermal energy at the operative conditions, nucleation occurs on the nanosecond timescale, which has been also confirmed by direct simulations [7]. Hence, one is interested in identifying the local supersaturation value $\sigma = c/c_{sat} - 1$, with $c$ and $c_{sat}$ the local and saturation gas concentration, respectively, at which the nucleation barrier $\Delta G^\dagger \leq 5$, and whether this concentration is achieved at the water/PFC interface. In the case of **homogeneous** supersaturated systems the barrier for nucleating a (spherical) bubble can be approximated by $\Delta G^\dagger = 16/3\pi(\gamma_0 + \sigma b)^3/(\sigma P)^3$, where $\gamma_0$ is the surface tension of the pure liquid, $b = -8.5 \times 10^{-5}$ N/(m atm) is the coefficient of reduction of the surface tension as a function of the pressure [8], the pressure being implicitly set to 1 bar and the effect of gas concentration taken into account by $\sigma$; finally, $P = 20$ MPa is the driving force for

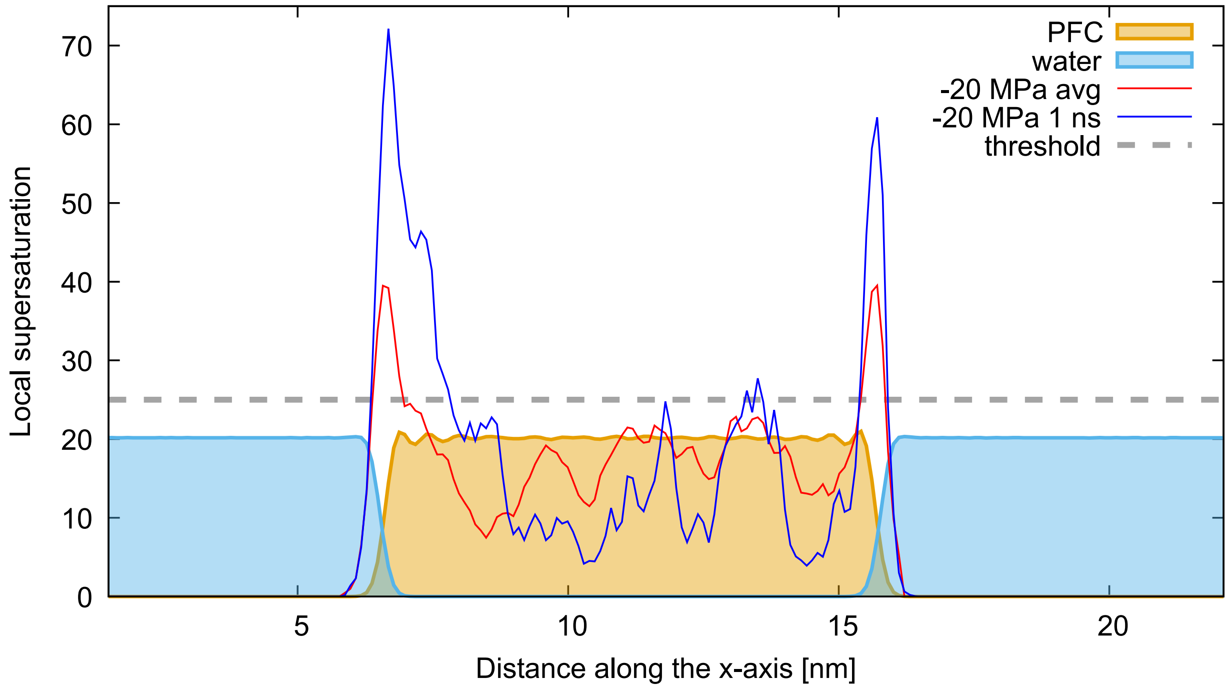


FIG. S 5. Local supersaturation of $N_2$ gas at $-20$ MPa with respect to the saturation value of nitrogen in water at ambient conditions. In the figure are reported both the supersaturation profile averaged over the entire simulation and the one averaged over 1 ns in which the local supersaturation value at the water/PFC interface was specially high. The grey dashed line is the threshold supersaturation value making the nucleation barrier small enough that the process could be experimentally observed.

bubble nucleation at the operative conditions of our experiments ($-20$ MPa of the Lamb-type wave). Usually, nucleation in heterogeneous conditions is taken into account through a reduction of this barrier by a multiplicative parameter that for a solid surface reads $\Phi(\theta) = 1/4(1+\cos\theta)^2(2-\cos\theta)$, with $\theta$ the contact angle of the liquid: $\Delta G^{\dagger}_{het} = \Delta G^{\dagger}_{homo}\Phi(\theta)$. Here, we develop or argument in the most conservative conditions, i. e., considering the case of homogeneous nucleation. Within this framework, and data reported in Ref. [8], one obtains the following values of the **homogeneous** nucleation barrier (expressed in $k_BT$ units):

| $\sigma$ | $\Delta G^{\dagger}/k_BT$ |
|---|---|
| 0.1 | $\sim 4 \times 10^5$ |
| 1 | $\sim 4 \times 10^3$ |
| 10 | $\sim 40$ |
| 25 | $\sim 5$ |
| 50 | $\sim 1.$ |

These results show that for $\sigma \gtrsim 25$ nucleation can occur at the operative conditions of our exper-

iments. As mentioned above, the heterogeneity introduced by the hydrophobic PFOB is expected to reduce local supersaturation necessary to produce bubble nucleation.

Generally speaking, obtaining $\sigma \gtrsim 25$ is non-trivial. However, one notices that the gas concentration at the water/PFOB is much larger than this threshold (see Fig. S5). In fact, nitrogen reaches a local density up to $\sim 2.5$ g/l concentration in the interface region, against a saturation concentration in water at normal conditions of $\sim 0.02$ g/l. Moreover, one must consider that local supersaturation may have fluctuations and for short times can reach much higher values. To illustrate this, in Fig. S5 we also report a supersaturation profile averaged over only 1 ns along the MD trajectory when its value at the water/PFC was especially high.

## VI. ADEQUACY OF THE SIZE OF THE COMPUTATIONAL SAMPLE

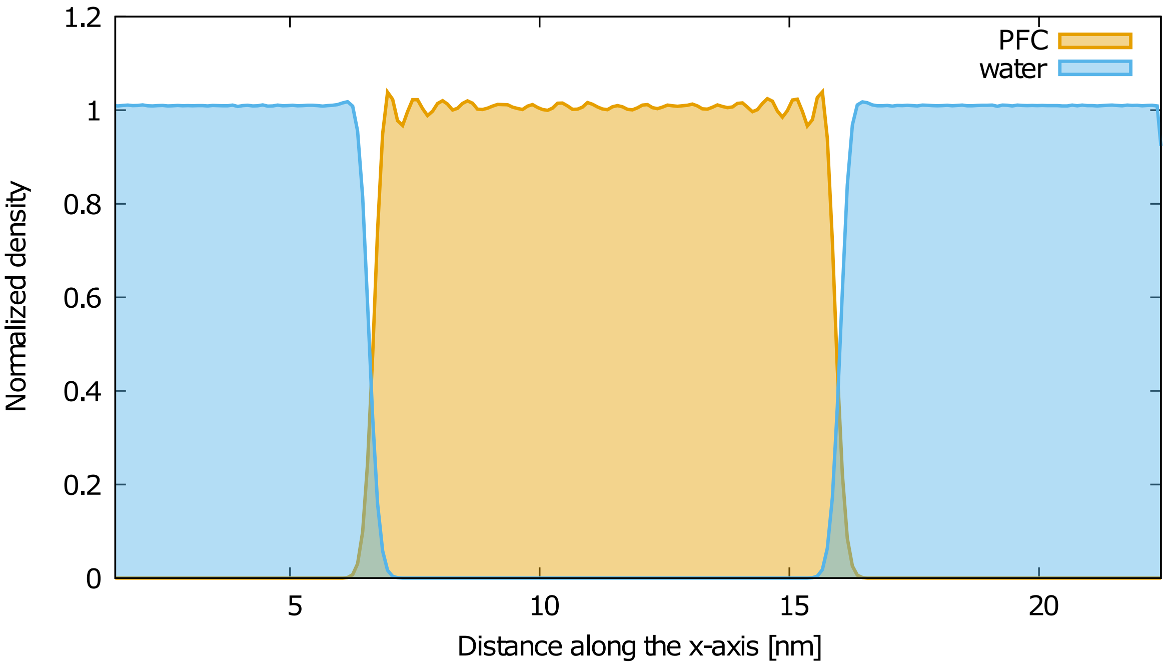


FIG. S 6. Density profile of the liquids, water (cyan) and PFC (yellow), along the axis transverse to the liquid/liquid interface.

For the computational sample to be suitable for the simulations of a gas at the water/PFOB, both liquid domains must be large enough that the bulk characteristics are recovered. Indeed, the normalized density profiles shown in Fig. 2 of the main text, reproduced in Fig. S6 without the gas density profiles, show within $\sim 1-2$ nm from the nominal interface, where the normalized densities of the two liquids are the same. There is first a depletion zone, where the density is lower than the bulk value, followed by a region in which gas density increases, and then a *rippling* region, where the densities oscillate around the

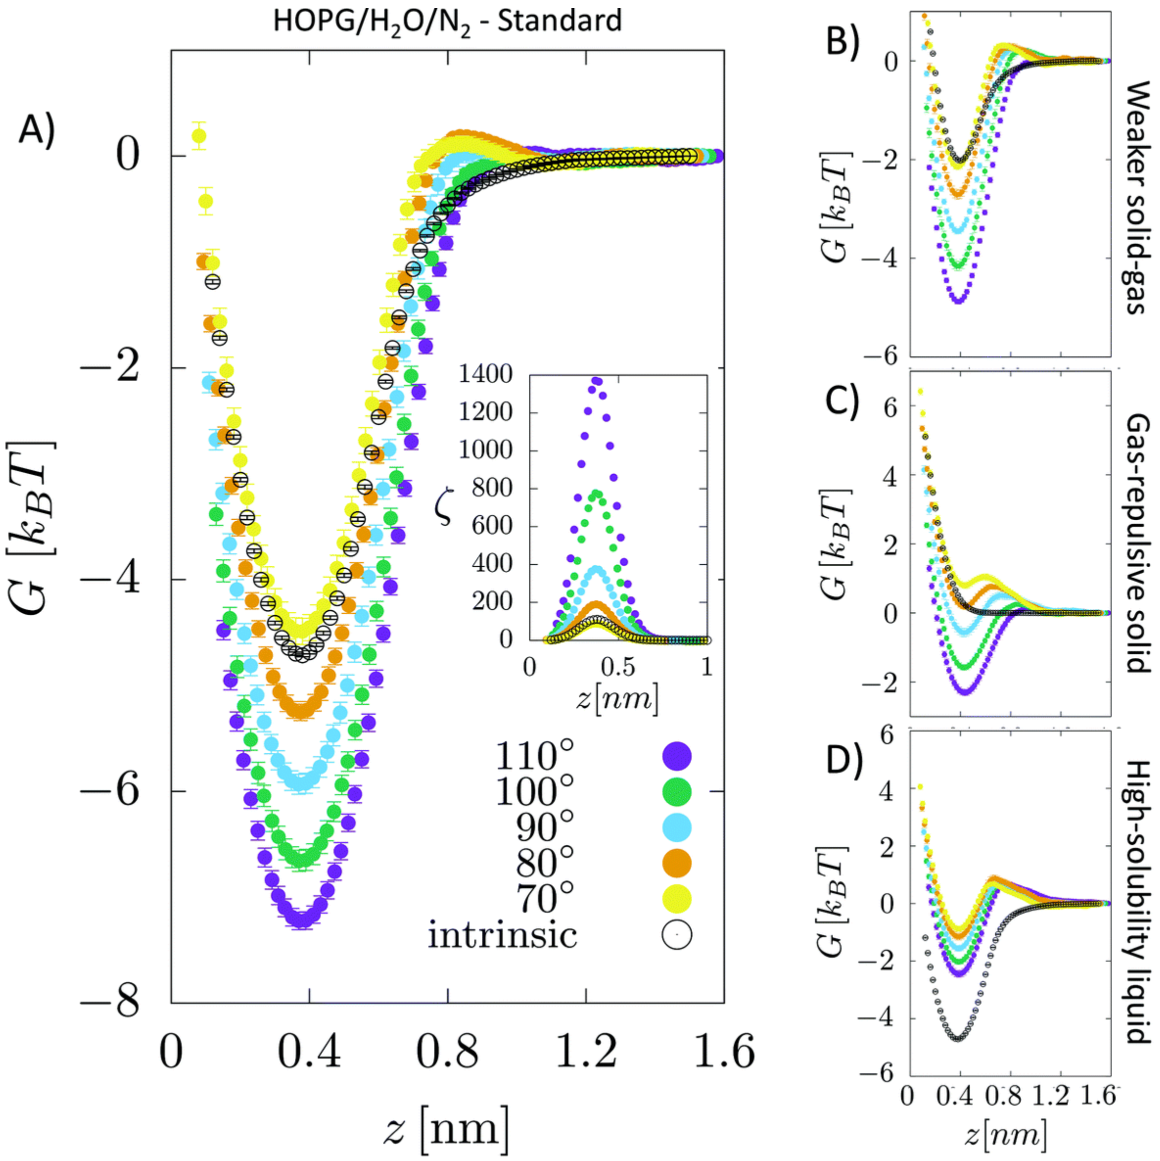


FIG. S 7. Effective potential between $N_2$ gas molecules in water as a function of the distance from a graphene sheet. Here, by *effective potential* one means the so-called potential of the mean force, obtained by restrained MD simulations [7, 9]. The effective potential depends on many factors, including the hydrophobicity of the solid, the strength of the gas-solid interaction and the strength of the gas-liquid interaction. Panels A to D show that regardless of these details, the range of the effective potential is on the nanometric scale, with the $N_2$ molecule subjected to a flat effective potential for distance from the interface $\geq 1$ nm. This means that beyond 1 nm from the interface the liquid is bulk-like for what concerns the gas properties. Error bars have been computed using the Jackknife resampling method using a sample size of 100 elements extracted along the molecular dynamics. Figure reprinted with permission from Ref. [9].

bulk value. These two phenomena are typical for liquids in contact with lyophobic surfaces, i. e., surfaces repelling the liquid, with a contact angle $\theta \geq 90°$. Indeed, this is consistent with the non miscibility of the two liquids. Beyond $2-3$ nm from the interface, however, the density profile of both liquids is

essentially flat, with small fluctuation due to the finite duration of MD simulations, which is long on the atomistic timescale but insufficient to sample the configurations space. This is especially visible in the case of PFC, which due to entanglement of longer molecules make the sampling especially difficult.

The above analysis can be made more quantitative resorting to the results of Ref. [9]. In this former article we computed the effective potential felt by gas molecules, $N_2$ and $O_2$, as a function of the distance from a graphene surface immersed in water. It is worth remarking that this effective potential does not only depend on the mechanical (force field - *intrinsic* in Fig. S7) solid-gas interaction. Instead in Fig. S7/A (reproduced with permission from Ref. [9]), it is seen that for the same graphene/$N_2$ mechanical interaction, the effective potential depends on the hydrophobicity of the interface. Indeed, the graphene/$N_2$ effective interaction can be attractive even if the corresponding mechanical interaction is weaker (Fig. S7/B) or purely repulsive (Fig. S7/C). Finally, the strength of the graphene/$N_2$ interaction depends on the affinity of the gas for liquid molecules. The reason why the interface is an attractive region for the gas is that there liquid is depleted. As a result this region favors to host the gas. Its attraction increases with the degree of depletion for example by an increase in hydrophobicity. The depletion region may decrease with in increase in gas solubility in the liquid. Overall we want to stress here that: i) The length scale of the attractive interaction is $\sim 1\,\mathrm{nm}$, which is the scale where the liquid density shows depletion and rippling. ii) The non-bulk like density field is found only within $\sim 2\,\mathrm{nm}$ of the water/PFC interface. This supports the choice of the size of our simulation, where each liquid domain is considerably larger.

---


[1] Battino, R., Rettich, T. R. & Tominaga, T. The Solubility of Nitrogen and Air in Liquids. *J. Phys. Chem. Ref. Data* **13**, 563–600 (1984).

[2] Lubetkin, S. D. Why is it much easier to nucleate gas bubbles than theory predicts? *Langmuir* **19**, 2575–2587 (2003).

[3] Kramers, H. A. Brownian motion in a field of force and the diffusion model of chemical reactions. *Physica* **7**, 284–304 (1940).

[4] Schulten, K., Schulten, Z. & Szabo, A. Dynamics of reactions involving diffusive barrier crossing. *The Journal of Chemical Physics* **74**, 4426–4432 (1981).

[5] Blander, M. & Katz, J. L. Bubble nucleation in liquids. *AIChE Journal* **21**, 833–848 (1975).

[6] Menzl, G. *et al.* Molecular mechanism for cavitation in water under tension. *Proceedings of the National Academy of Sciences* **113**, 13582–13587 (2016).

[7] Lisi, E., Amabili, M., Meloni, S., Giacomello, A. & Casciola, C. M. Self-recovery superhydrophobic surfaces: Modular design. *ACS nano* **12**, 359–367 (2018).

[8] Massoudi, R. & King Jr, A. Effect of pressure on the surface tension of water. adsorption of low molecular weight gases on water at 25. deg. *The Journal of Physical Chemistry* **78**, 2262–2266 (1974).

[9] Tortora, M. *et al.* The interplay among gas, liquid and solid interactions determines the stability of surface nanobubbles. *Nanoscale* **12**, 22698–22709 (2020).
